# Supplementary material for: LeForecast: Enterprise Hybrid Forecast by Time Series Intelligence
Source: arXiv:2503.22747 source file (2025-03-27)
Supplement: Supplementary file 1 [file appendix-a.tex]

%%%%%%%%%%%%%%%%%%%%%%%%%%%%%%%%%%%%%%%%%
%%% Appendix A. Achievements and Awards
%%%%%%%%%%%%%%%%%%%%%%%%%%%%%%%%%%%%%%%%%

\section{Achievements}
%\addcontentsline{toc}{section}{Achievements}
\label{sec:appendix-a}

\subsection{Patents}
\label{sec:appendix-a-patent}
%\addcontentsline{toc}{subsection}{A.1. Patents}

\subsection{Papers}
\label{sec:appendix-a-papers}
% \addcontentsline{toc}{subsection}{A.2. Papers}

\subsection{Awards}
\label{sec:appendix-a-awards}
% \addcontentsline{toc}{subsection}{A.3. Awards}
