# Supplementary material for: LeForecast: Enterprise Hybrid Forecast by Time Series Intelligence
Source: arXiv:2503.22747 source file (2025-03-27)
Supplement: Supplementary file 2 [file appendix-b.tex]

%%%%%%%%%%%%%%%%%%%%%%%%%%%%%%%%%%%%%%%%%
%%% Appendix B. Prompts
%%%%%%%%%%%%%%%%%%%%%%%%%%%%%%%%%%%%%%%%%

% \clearpage
% \section{Data Portfolio}
% % \addcontentsline{toc}{section}{Appendix B. Prompts}
% \label{sec:appendix-b}

% \subsection{Data Statistics}
% \label{sec:appendix-b-websearch}
% % \addcontentsline{toc}{subsection}{B.1. Web Search for News Agent}

% \subsection{Statistics of Training Datasets}
% \label{sec:appendix-b-data}
% % \addcontentsline{toc}{subsection}{B.2. Data Analysis for Data Agent}

% \subsection{Examples of Synthetic Data}
% \label{sec:appendix-b-report}
% % \addcontentsline{toc}{subsection}{B.3. Report Summary for Report Agent}

%%%%%%%%%%%%%%%%%%%%%%%%%%%%%%%%%%%%%%%%%
